# Supplementary material for: Effortless Data Exploration with zenvisage: An Expressive and Interactive Visual Analytics System
Source: arXiv:1604.03583 source file (2018-01-04)
Supplement: Supplementary file 3 [file queryexec-appendix.tex]

\section{Query Execution: Naive Translation Listing}
\label{queryexec-appendix}

Here, we list the pseudocode for the naive translation 
for query execution for reference.
{
\begin{lstlisting}[columns=fullflexible,basicstyle=\ttfamily,
  caption={Pseudocode for the compiled query in Table~\ref{tab:exec-1}},label={lst:exec-1}]
# Row 1
v1_range = P,
f1 = make_array(1, size(v1_range))
for v1 in [0 .. size(v1_range)]:
  f1[v1] = sql(``SELECT year, SUM(sales)
                WHERE product=`%s' and location=`US'
                GROUP BY year ORDER BY year''),
              v1_range[v1])
v2_range = []
for v1 in [0 .. size(v1_range)]:
  if T(f1[v1]) > 0:
    v2_range.append(v1_range[v1])

# Row 2
f2 = make_array(1, size(v1_range))
for v1 in [0 .. size(v1_range)]:
  f2[v1] = sql(``SELECT year, SUM(sales)
                WHERE product=`%s' and location=`UK'
                GROUP BY year ORDER BY year''),
              v1_range[v1])
v3_range = []
for v1 in [0 .. size(v1_range)]:
  if T(f2[v1]) < 0:
    v3_range.append(v1_range[v1])

# Row 3
v4_range = union(v2_range, v3_range)
f3 = make_array(1, size(v4_range))
for v4 in [0 .. size(v4_range)]:
  f3[v4] = sql(``SELECT year, SUM(profit)
                WHERE product=`%s'
                GROUP BY year ORDER BY year''),
              v4_range[v4])

return f3
\end{lstlisting}
}
